# Supplementary material for: dFlowGRPO: Rate-Aware Policy Optimization for Discrete Flow Models
Source: arXiv:2605.09291 source file (2026-10-01)
Supplement: Supplementary file 1 [file appendix_additional_experiments.tex]

\section{Additional experimental results}
